# Supplementary material for: Prospects for $B_c^+$ and $B^+\to \tau^+ \nu_\tau$ at FCC-ee
Source: arXiv:2305.02998 source file (2024-05-15)
Supplement: Supplementary file 1 [file appendix.tex]

\clearpage
\appendix

\section{BDT training variable distributions}
\label{app:bdt_vars}

\begin{figure}[h!]
\centering
\includegraphics[width = 0.22\textwidth]{figs/Bc2TauNu_vs_inclusive_Z_uds_cc_bb_EVT_ThrustEmin_E_vtx.pdf}
\includegraphics[width = 0.22\textwidth]{figs/Bc2TauNu_vs_inclusive_Z_uds_cc_bb_EVT_ThrustEmax_E_vtx.pdf}
\includegraphics[width = 0.22\textwidth]{figs/Bc2TauNu_vs_inclusive_Z_uds_cc_bb_EVT_ThrustEmin_Echarged_vtx.pdf} 
\includegraphics[width = 0.22\textwidth]{figs/Bc2TauNu_vs_inclusive_Z_uds_cc_bb_EVT_ThrustEmax_Echarged_vtx.pdf} \\
\includegraphics[width = 0.22\textwidth]{figs/Bc2TauNu_vs_inclusive_Z_uds_cc_bb_EVT_ThrustEmin_Eneutral_vtx.pdf}
\includegraphics[width = 0.22\textwidth]{figs/Bc2TauNu_vs_inclusive_Z_uds_cc_bb_EVT_ThrustEmax_Eneutral_vtx.pdf}
\includegraphics[width = 0.22\textwidth]{figs/Bc2TauNu_vs_inclusive_Z_uds_cc_bb_EVT_ThrustEmin_Ncharged_vtx.pdf}
\includegraphics[width = 0.22\textwidth]{figs/Bc2TauNu_vs_inclusive_Z_uds_cc_bb_EVT_ThrustEmax_Ncharged_vtx.pdf} \\
\includegraphics[width = 0.22\textwidth]{figs/Bc2TauNu_vs_inclusive_Z_uds_cc_bb_EVT_ThrustEmin_Nneutral_vtx.pdf}
\includegraphics[width = 0.22\textwidth]{figs/Bc2TauNu_vs_inclusive_Z_uds_cc_bb_EVT_ThrustEmax_Nneutral_vtx.pdf}
\includegraphics[width = 0.22\textwidth]{figs/Bc2TauNu_vs_inclusive_Z_uds_cc_bb_EVT_NtracksPV_vtx.pdf}
\includegraphics[width = 0.22\textwidth]{figs/Bc2TauNu_vs_inclusive_Z_uds_cc_bb_EVT_NVertex_vtx.pdf} \\
\includegraphics[width = 0.22\textwidth]{figs/Bc2TauNu_vs_inclusive_Z_uds_cc_bb_EVT_NTau23Pi_vtx.pdf}
\includegraphics[width = 0.22\textwidth]{figs/Bc2TauNu_vs_inclusive_Z_uds_cc_bb_EVT_ThrustEmin_NDV_vtx.pdf} 
\includegraphics[width = 0.22\textwidth]{figs/Bc2TauNu_vs_inclusive_Z_uds_cc_bb_EVT_ThrustEmax_NDV_vtx.pdf} 
\includegraphics[width = 0.22\textwidth]{figs/Bc2TauNu_vs_inclusive_Z_uds_cc_bb_EVT_dPV2DVmin_vtx.pdf}  \\
\includegraphics[width = 0.22\textwidth]{figs/Bc2TauNu_vs_inclusive_Z_uds_cc_bb_EVT_dPV2DVmax_vtx.pdf} 
\includegraphics[width = 0.22\textwidth]{figs/Bc2TauNu_vs_inclusive_Z_uds_cc_bb_EVT_dPV2DVave_vtx.pdf} 
\caption{First-stage BDT training variable distributions in signal, $B^+ \to \tau^+ \nu_\tau$ background, and inclusive $Z^0 \to q\bar{q},c\bar{c},b\bar{b}$ background.}
\label{fig:BDT1_vars}
\end{figure}

\begin{figure}[h!]
\centering
\includegraphics[width = 0.22\textwidth]{figs/Bc2TauNu_vs_inclusive_Z_uds_cc_bb_EVT_CandMass_stage2.pdf}
\includegraphics[width = 0.22\textwidth]{figs/Bc2TauNu_vs_inclusive_Z_uds_cc_bb_EVT_CandRho1Mass_stage2.pdf}
\includegraphics[width = 0.22\textwidth]{figs/Bc2TauNu_vs_inclusive_Z_uds_cc_bb_EVT_CandRho2Mass_stage2.pdf}
\includegraphics[width = 0.22\textwidth]{figs/Bc2TauNu_vs_inclusive_Z_uds_cc_bb_EVT_CandN_stage2.pdf} \\
\includegraphics[width = 0.22\textwidth]{figs/Bc2TauNu_vs_inclusive_Z_uds_cc_bb_EVT_CandVtxFD_stage2.pdf}
\includegraphics[width = 0.22\textwidth]{figs/Bc2TauNu_vs_inclusive_Z_uds_cc_bb_EVT_CandVtxChi2_stage2.pdf}
\includegraphics[width = 0.22\textwidth]{figs/Bc2TauNu_vs_inclusive_Z_uds_cc_bb_EVT_CandPx_stage2.pdf}
\includegraphics[width = 0.22\textwidth]{figs/Bc2TauNu_vs_inclusive_Z_uds_cc_bb_EVT_CandPy_stage2.pdf} \\
\includegraphics[width = 0.22\textwidth]{figs/Bc2TauNu_vs_inclusive_Z_uds_cc_bb_EVT_CandPz_stage2.pdf} 
\includegraphics[width = 0.22\textwidth]{figs/Bc2TauNu_vs_inclusive_Z_uds_cc_bb_EVT_CandP_stage2.pdf}
\includegraphics[width = 0.22\textwidth]{figs/Bc2TauNu_vs_inclusive_Z_uds_cc_bb_EVT_CandD0_stage2.pdf}
\includegraphics[width = 0.22\textwidth]{figs/Bc2TauNu_vs_inclusive_Z_uds_cc_bb_EVT_CandZ0_stage2.pdf} \\
\includegraphics[width = 0.22\textwidth]{figs/Bc2TauNu_vs_inclusive_Z_uds_cc_bb_EVT_CandAngleThrust_stage2.pdf} 
\includegraphics[width = 0.22\textwidth]{figs/Bc2TauNu_vs_inclusive_Z_uds_cc_bb_EVT_DVd0_min_stage2.pdf} 
\includegraphics[width = 0.22\textwidth]{figs/Bc2TauNu_vs_inclusive_Z_uds_cc_bb_EVT_DVd0_max_stage2.pdf} 
\includegraphics[width = 0.22\textwidth]{figs/Bc2TauNu_vs_inclusive_Z_uds_cc_bb_EVT_DVd0_ave_stage2.pdf} \\
\includegraphics[width = 0.22\textwidth]{figs/Bc2TauNu_vs_inclusive_Z_uds_cc_bb_EVT_DVz0_min_stage2.pdf} 
\includegraphics[width = 0.22\textwidth]{figs/Bc2TauNu_vs_inclusive_Z_uds_cc_bb_EVT_DVz0_max_stage2.pdf} 
\includegraphics[width = 0.22\textwidth]{figs/Bc2TauNu_vs_inclusive_Z_uds_cc_bb_EVT_DVz0_ave_stage2.pdf} 
\includegraphics[width = 0.22\textwidth]{figs/Bc2TauNu_vs_inclusive_Z_uds_cc_bb_EVT_PVmass_stage2.pdf} \\
\includegraphics[width = 0.22\textwidth]{figs/Bc2TauNu_vs_inclusive_Z_uds_cc_bb_EVT_Nominal_B_E_stage2.pdf} 

\caption{Second-stage BDT training variable distributions in signal, $B^+ \to \tau^+ \nu_\tau$ background, and inclusive $Z^0 \to q\bar{q},c\bar{c},b\bar{b}$ background.}
\label{fig:BDT2_vars}
\end{figure}

\FloatBarrier

\section{Exclusive background efficiencies}
\label{app:bkg_effs}

{
\begin{table}[h!]
\centering
\scriptsize
\begin{tabular}{lllll}
Decay mode & N(expected) & N(generated) & Expected / Generated & Final $\epsilon$ \\ \hline
$B^+ \to \bar{D}^0 \tau^+ \nu_\tau$ & $5.01 \times 10^{9}$ & $2 \times 10^{8}$ & $25.0$ & $1.46 \times 10^{-9}$ \\
$B^+ \to \bar{D}^{*0} \tau^+ \nu_\tau$ & $1.22 \times 10^{10}$ & $2 \times 10^{8}$ & $61.1$ & $1.1 \times 10^{-9}$ \\
$B^+ \to \bar{D}^0 3\pi$ & $3.64 \times 10^{9}$ & $1.9 \times 10^{8}$ & $19.2$ & $1.56 \times 10^{-9}$ \\
$B^+ \to \bar{D}^{*0} 3\pi$ & $6.7 \times 10^{9}$ & $2 \times 10^{8}$ & $33.5$ & $1.04 \times 10^{-9}$ \\
$B^+ \to \bar{D}^0 D_s^+$ & $5.85 \times 10^{9}$ & $2 \times 10^{8}$ & $29.3$ & $2.52 \times 10^{-10}$ \\
$B^+ \to \bar{D}^{*0} D_s^+$ & $4.94 \times 10^{9}$ & $1.75 \times 10^{8}$ & $28.2$ & $2.72 \times 10^{-10}$ \\
$B^+ \to \bar{D}^{*0} D_s^{*+}$ & $1.11 \times 10^{10}$ & $2 \times 10^{8}$ & $55.6$ & $2.42 \times 10^{-10}$ \\
\hline
$B^0 \to D^- \tau^+ \nu_\tau$ & $7.02 \times 10^{9}$ & $2 \times 10^{8}$ & $35.1$ & $2.69 \times 10^{-9}$ \\
$B^0 \to D^{*-} \tau^+ \nu_\tau$ & $1.02 \times 10^{10}$ & $2 \times 10^{8}$ & $51.0$ & $1.25 \times 10^{-9}$ \\
$B^0 \to D^- 3\pi$ & $3.9 \times 10^{9}$ & $2 \times 10^{8}$ & $19.5$ & $3.4 \times 10^{-9}$ \\
$B^0 \to D^{*-} 3\pi$ & $4.69 \times 10^{9}$ & $2 \times 10^{8}$ & $23.4$ & $9.84 \times 10^{-10}$ \\
$B^0 \to D^- D_s^+$ & $4.68 \times 10^{9}$ & $2 \times 10^{8}$ & $23.4$ & $3.23 \times 10^{-10}$ \\
$B^0 \to D^{*-} D_s^+$ & $5.2 \times 10^{9}$ & $2 \times 10^{8}$ & $26.0$ & $2.32 \times 10^{-10}$ \\
$B^0 \to D^{*-} D_s^{*+}$ & $1.15 \times 10^{10}$ & $2 \times 10^{8}$ & $57.5$ & $2.35 \times 10^{-10}$ \\
\hline
$B_s^0 \to D_s^- \tau^+ \nu_\tau$ & $3.53 \times 10^{9}$ & $2 \times 10^{8}$ & $17.6$ & $3.71 \times 10^{-9}$ \\
$B_s^0 \to D_s^{*-} \tau^+ \nu_\tau$ & $2.35 \times 10^{9}$ & $2 \times 10^{8}$ & $11.8$ & $2.27 \times 10^{-9}$ \\
$B_s^0 \to D_s^- 3\pi$ & $8.85 \times 10^{8}$ & $2 \times 10^{8}$ & $4.4$ & $5.53 \times 10^{-9}$ \\
$B_s^0 \to D_s^{*-} 3\pi$ & $1.05 \times 10^{9}$ & $2 \times 10^{8}$ & $5.2$ & $3.38 \times 10^{-9}$ \\
$B_s^0 \to D_s^- D_s^+$ & $6.39 \times 10^{8}$ & $2 \times 10^{8}$ & $3.2$ & $4.09 \times 10^{-10}$ \\
$B_s^0 \to D_s^{*-} D_s^+$ & $2.02 \times 10^{9}$ & $2 \times 10^{8}$ & $10.1$ & $3.17 \times 10^{-10}$ \\
$B_s^0 \to D_s^{*-} D_s^{*+}$ & $2.09 \times 10^{9}$ & $2 \times 10^{8}$ & $10.5$ & $2.56 \times 10^{-10}$ \\
\hline
$\Lambda_b^0 \to \Lambda_c^- \tau^+ \nu_\tau$ & $1.83 \times 10^{9}$ & $2 \times 10^{8}$ & $9.1$ & $1.36 \times 10^{-9}$ \\
$\Lambda_b^0 \to \Lambda_c^{*-} \tau^+ \nu_\tau$ & $1.83 \times 10^{9}$ & $2 \times 10^{8}$ & $9.1$ & $9.44 \times 10^{-10}$ \\
$\Lambda_b^0 \to \Lambda_c^- 3\pi$ & $4.31 \times 10^{8}$ & $2 \times 10^{8}$ & $2.2$ & $5.58 \times 10^{-9}$ \\
$\Lambda_b^0 \to \Lambda_c^{*-} 3\pi$ & $4.31 \times 10^{8}$ & $2 \times 10^{8}$ & $2.2$ & $9.21 \times 10^{-10}$ \\
$\Lambda_b^0 \to \Lambda_c^- D_s^+$ & $6.15 \times 10^{8}$ & $2 \times 10^{8}$ & $3.1$ & $3.46 \times 10^{-10}$ \\
$\Lambda_b^0 \to \Lambda_c^{*-} D_s^+$ & $6.15 \times 10^{8}$ & $2 \times 10^{8}$ & $3.1$ & $2.72 \times 10^{-10}$ \\
$\Lambda_b^0 \to \Lambda_c^{*-} D_s^{*+}$ & $6.15 \times 10^{8}$ & $2 \times 10^{8}$ & $3.1$ & $2.5 \times 10^{-10}$ \\
\hline
\end{tabular}
\caption{Summary of the exclusive $B$-hadron background samples used for determination of the optimal BDT cuts and to model background in the signal yield fit. The yields expected for each decay mode with $N_Z = 5 \times 10^{12}$ are shown in the second column, and the generated sample statistics are shown in the third column. The large ratio between expected and generated statistics (fourth column) illustrates why cut-and-count efficiencies cannot be used to determine the expected background rejection achieved by the double-BDT selection; for many background modes, none of the generated events survive the optimal BDT cuts applied. The efficiency values determined using the spline parameterisation approach are given in the final column. Using splines derived from the total exclusive sample enables efficiencies down to the $10^{-10}$ level to be evaluated.}
\label{tab:bkg_BDT_effs}
\end{table}
}

\FloatBarrier

\newpage

\section{Signal yield and branching fraction precision estimates}
\label{app:precisions}

{
\begin{table}[h!]
\centering
\small
\begin{tabular}{ll}
$N_Z (\times 10^{12})$ & Relative $\sigma$ ($\sigma_{syst}^N = [0, 0.25, 0.5, 1] \times \sigma_{stat}^N$) \\ \hline
0.5 & [0.078, 0.087, 0.096, 0.111] \\
1 & [0.055, 0.061, 0.067, 0.077] \\
2 & [0.038, 0.042, 0.046, 0.053] \\
3 & [0.032, 0.036, 0.039, 0.046] \\
4 & [0.027, 0.03, 0.033, 0.038] \\
5 & [0.024, 0.027, 0.03, 0.034] \\
\hline
\end{tabular}
\caption{Estimated relative precision on $N(B_c^+ \to \tau^+ \nu_\tau)$ as a function of $N_Z$, where four different levels of systematic uncertainty on the signal yield are shown.}
\label{tab:N_Bc2TauNu_vs_NZ}
\end{table}
}

{
\begin{table}[h!]
\centering
\small
\begin{tabular}{ll}
$N_Z (\times 10^{12})$ & Relative $\sigma$ ($\sigma_{syst}^N = [0, 0.25, 0.5, 1] \times \sigma_{stat}^N$) \\ \hline
0.5 & [0.081, 0.09, 0.098, 0.113] \\
1 & [0.058, 0.064, 0.07, 0.08] \\
2 & [0.042, 0.046, 0.05, 0.056] \\
3 & [0.037, 0.04, 0.043, 0.049] \\
4 & [0.032, 0.035, 0.037, 0.042] \\
5 & [0.03, 0.032, 0.034, 0.038] \\
\hline
\end{tabular}
\caption{Estimated relative precision on $\mathcal{R}$ as a function of $N_Z$, where four different levels of systematic uncertainty on the signal yield are shown.}
\label{tab:BF_ratio_vs_NZ}
\end{table}
}

{
\begin{table}[h!]
\centering
\small
\begin{tabular}{ll}
$N_Z (\times 10^{12})$ & Relative $\sigma$ ($\sigma_{syst}^N = [0, 0.25, 0.5, 1] \times \sigma_{stat}^N$) \\ \hline
0.5 & [0.115, 0.122, 0.128, 0.139] \\
1 & [0.1, 0.104, 0.107, 0.114] \\
2 & [0.092, 0.093, 0.095, 0.099] \\
3 & [0.089, 0.091, 0.092, 0.095] \\
4 & [0.088, 0.089, 0.09, 0.092] \\
5 & [0.087, 0.088, 0.088, 0.09] \\
\hline
\end{tabular}
\caption{Estimated relative precision on $\mathcal{B}(B_c^+ \to \tau^+ \nu_\tau)$ as a function of $N_Z$, where four different levels of systematic uncertainty on the signal yield are shown.}
\label{tab:BF_Bc2TauNu_vs_NZ}
\end{table}
}

\FloatBarrier
